# Supplementary material for: Investigating the Interplay between Features and Structures in Graph Learning
Source: arXiv:2308.09570 source file (2023-08-18)
Supplement: Supplementary file 1 [file appendix.tex]

\section{Experiments Details}

\subsubsection{Model Selection.}
